# Supplementary material for: On the Computational Landscape of Replicable Learning
Source: arXiv:2405.15599 source file (2024-11-30)
Supplement: Supplementary file 1 [file appendix.tex]

\input{lifting_gaps}
